# Supplementary material for: PT-Mark: Invisible Watermarking for Text-to-image Diffusion Models via Semantic-aware Pivotal Tuning
Source: arXiv:2504.10853 source file (2025-04-18)
Supplement: Supplementary file 1 [file 7_appendix.tex]

\appendix
\section{Appendix}

\subsection{Quantitative Evaluation of Real-world Adaptive Attacks}
\label{sec:adaptive_attack}

In this section, we evaluate the robustness of PT-Mark against real-world adaptive watermark removal attacks. We consider three typical watermark removal attack methods: Bmshj18~\cite{Bmshj18}, Cheng20~\cite{Cheng20}, which use a VAE-based image compression model with a quality level of 3 to remove watermark patterns, and Zhao23~\cite{Zhao23}, which leverages a stable diffusion model to regenerate the watermarked image with 60 denoising steps.
The evaluation results are presented in Table~\ref{table:adaptive_attack}. We demonstrate that PT-Mark achieves the highest robustness compared to state-of-the-art methods, maintaining 100\% watermark verification accuracy. Notably, we observe that traditional watermarking methods experience a significant decrease in accuracy when faced with these real-world adaptive attacks.

% In this section, we evaluate the robustness of PT-Mark under real-world adaptive watermark removal attackers. We consider three typical real-world watermark removal attack methods: 
% Bmshj18[] and Cheng20[], which takes VAE-based image compression model to removal the watermark patterns, and Zhao23[], which leverages a stable diffusion model to regrenerate the watermarked image with 60 denoising steps.
% The evaluation results are presented in Table~\ref{table:adaptive_attack}.
% We show that PT-Mark exhibits the highest robustness compared to the state-of-the-art, achieving 100\% watermark verification accuracy. 
% Notably, we find that traditional watermarking methods show severe decrease in accuracy when confronted to these real-world adaptive attacks. 

% \begin{table}[h!]
% \centering
% \begin{tabular}{l|c|c|c}
% \hline
% \textbf{Watermarking Method} & \textbf{Bmshj18} & \textbf{Cheng20} & \textbf{Zhao23} \\
% \hline
% DwtDct & 0.49 & 0.48 & 0.49 \\
% DwtDctSvc & 0.53 & 0.54 & 0.58 \\
% RivaGAN & 0.54 & 0.54 & 0.59 \\
% StegaStam & 1.00 & 1.00 & 0.93 \\
% Tree-ring & 1.00 & 1.00 & 1.00 \\
% ROBIN & 1.00 & 1.00 & 1.00 \\
% Zodiac & 0.91 & 0.94 & 0.90 \\
% \rowcolor[gray]{0.9}Ours & 1.00 & 1.00 & 1.00 \\
% \hline
% \end{tabular}
% \caption{Quantitative evaluation of different watermarking methods against real-world watermark removal attacks.}
% \end{table}

\begin{table}[h]
\centering
\resizebox{\columnwidth}{!}{
\begin{tabular}{l|c|c|c}
\hline
\multirow{2}{*}{\textbf{Watermarking Method}} & \multicolumn{3}{c}{\textbf{Attack Methods}} \\
\cline{2-4}
& \textbf{Bmshj18~\cite{Bmshj18}} & \textbf{Cheng20~\cite{Cheng20}} & \textbf{Zhao23~\cite{Zhao23}} \\
\hline
DwtDct & 0.49 & 0.48 & 0.49 \\
DwtDctSvc & 0.53 & 0.54 & 0.58 \\
RivaGAN & 0.54 & 0.54 & 0.59 \\
StegaStam & 1.00 & 1.00 & 0.93 \\
Tree-ring & 1.00 & 1.00 & 1.00 \\
ROBIN & 1.00 & 1.00 & 1.00 \\
Zodiac & 0.91 & 0.94 & 0.90 \\
\rowcolor[gray]{0.9}Ours & 1.00 & 1.00 & 1.00 \\
\hline
\end{tabular}}
\caption{Quantitative evaluation of different watermarking methods against real-world watermark removal attacks.}
\label{table:adaptive_attack}
\end{table}

\subsection{Ablation Study of Hyperparameter}
In this section, we conduct an ablation study to investigate the hyperparameters $\lambda_{1}$ and $\lambda_{2}$, which balance the two training objectives presented in Equation~\ref{eq:all}. We present the results for $\lambda_{1}$ from \{ 0.50, 1.00, 1.50, 2.00\} and vary $\lambda_{2}$ from \{0.0003, 0.0005, 0.0007\} to identify an optimal trade-off between semantic maintenance and watermark preservation. 
The evaluation results are shown in Table~\ref{table:ablation_loss}. 
We show that modifying the hyperparameters results in only slight changes in the SSIM and MSSIM metrics. Therefore, we focus on selecting the hyperparameters based on the combination of PSNR and average watermark verification accuracy. Our results show that when $\lambda_{1} = 1.50, \lambda_{2} = 0.0007$, the method achieves the best performance in balancing robustness and image semantic preservation.
% In this section, we conduct the ablation study to investigate the hyperparameter $\lambda_{1}, \lambda_{2}$ to balance the two training objectives presented in Equation~\ref{eq:all}. We present the results of $\lambda_{1}=1$ and change $\lambda_{2}$ from 0.0001 to 1 to find a good trade-off between semantic maintainance and watermark preservation. 

\begin{table*}[h]
\centering
\begin{tabular}{l|c|c|c|c|c|c|c|c|c|c|c|c|c}
\hline
$\lambda_{1}$ & $\lambda_{2}$ & SSIM~($\uparrow$) & PSNR~($\uparrow$) & LPIPS~($\downarrow$) & MSSIM~($\uparrow$) & Clean & JPEG & Crop & Blur & Noise & Bright & Rotation & Avg \\
\hline
\multirow{3}{*}{0.50} & 0.0003 & 0.92 & 27.64 & 0.05 & 0.96 & 1.00 & 0.99 & 0.99 & 1.00 & 0.96 & 0.99 & 0.96 & 0.98 \\
 & 0.0005 & 0.92 & 26.94 & 0.05 & 0.96 & 1.00 & 1.00 & 1.00 & 1.00 & 1.00 & 1.00 & 0.96 & 0.99 \\
 & 0.0007 & 0.92 & 26.29 & 0.06 & 0.96 & 1.00 & 1.00 & 1.00 & 1.00 & 0.96 & 1.00 & 0.96 & 0.99 \\
\hline
\multirow{3}{*}{1.00} & 0.0003 & 0.94 & 28.58 & 0.04 & 0.97 & 1.00 & 0.97 & 0.97 & 1.00 & 0.90 & 0.97 & 0.94 & 0.96 \\
 & 0.0005 & 0.94 & 28.03 & 0.03 & 0.97 & 1.00 & 1.00 & 0.98 & 1.00 & 0.95 & 1.00 & 0.96 & 0.98 \\
 & 0.0007 & 0.93 & 27.63 & 0.05 & 0.96 & 1.00 & 1.00 & 1.00 & 1.00 & 0.96 & 1.00 & 0.97 & 0.99 \\
\hline
\multirow{3}{*}{1.50} & 0.0003 & 0.94 & 28.69 & 0.03 & 0.97 & 1.00 & 0.96 & 0.96 & 0.99 & 0.93 & 0.93 & 0.92 & 0.95 \\
 & 0.0005 & 0.94 & 28.48 & 0.03 & 0.97 & 1.00 & 1.00 & 1.00 & 1.00 & 0.94 & 1.00 & 0.96 & 0.98 \\
 & \rowcolor[gray]{0.9} 0.0007 & 0.94 & 28.18 & 0.03 & 0.97 & 1.00 & 1.00 & 0.98 & 1.00 & 0.96 & 1.00 & 0.97 & 0.99 \\
\hline
\multirow{3}{*}{2.00} & 0.0003 & 0.94 & 28.32 & 0.05 & 0.96 & 1.00 & 0.92 & 0.96 & 1.00 & 0.91 & 0.93 & 0.90 & 0.94 \\
 & 0.0005 & 0.94 & 28.76 & 0.03 & 0.97 & 1.00 & 0.96 & 1.00 & 1.00 & 0.94 & 1.00 & 0.96 & 0.98 \\
 & 0.0007 & 0.94 & 28.43 & 0.04 & 0.97 & 1.00 & 0.98 & 1.00 & 1.00 & 0.95 & 1.00 & 0.96 & 0.98 \\
\hline
\end{tabular}
\caption{Ablation study results for different loss weights $\lambda_{1}, \lambda_{2}$ across image quality metrics and robustness under varying real-world perturbations.}
\label{table:ablation_loss}
\end{table*}
